# Supplementary material for: Benchmarking Reinforcement Learning Techniques for Autonomous Navigation
Source: arXiv:2210.04839 source file (2023-06-27)
Supplement: Supplementary file 1 [file appendix_nav_env.tex]

\section{Navigation Benchmark}
\subsection{Comparison of Navigation Benchmark}
\rebuttal{See \ref{tab::related} for a comparison between existing navigation benchmarks.}
\begin{table}[htb!]
\resizebox{\columnwidth}{!}{%
\color{blue}\begin{tabular}{lccccc}
\toprule 
             & High-fidelity physics     & ROS integration           & Collision-free navigation & Photo-realism & Ground navigation\\
             \midrule 
iGibson~\cite{xia2020interactive}       & \Checkmark &\Checkmark & \XSolid & \Checkmark &  \Checkmark  \\
Mazeexplorer~\cite{harries2019mazeexplorer} & \XSolid    & \XSolid    & \XSolid & \XSolid &  \Checkmark \\
AI2-THOR~\cite{zhu2017target}  & \Checkmark  & \XSolid &  \XSolid & \Checkmark &  \Checkmark \\
Aquatic navigation~\cite{marchesini2021benchmarking} & \Checkmark & \XSolid & \Checkmark & \XSolid & \XSolid \\
BARN (ours)  & \Checkmark & \Checkmark & \Checkmark  &\XSolid &  \Checkmark \\
             \bottomrule
\end{tabular}%
}
\vspace{5pt}
\caption{The comparison between different navigation benchmarks in terms of high-fidelity physics, ROS integration, collision-free navigation, Photo-realism, and ground navigation.}
\label{tab::related}
\end{table}

\subsection{Navigation Environments}
\label{appendix:nav_env}
\textbf{Static environments.} We use the 300 static environments from the BARN dataset \cite{perille2020benchmarking}. The obstacle fields in these environments are represented by a 30$\times$30 black-white grid, which corresponds to an area of 4.5m$\times$4.5m with black and white cells representing obstacle-occupied and free space respectively (see Fig. \ref{fig:static}). The grid cells are generated by a method of cellular automation \cite{wolfram1983statistical}, which is originally designed to generate a collection of black cells on a white grid of specified shape that evolves through a number of discrete time steps according to a set of rules based on the states of neighboring cells. In BARN, such generation process begins with randomly filling the grid cells by a ratio of \textit{initial fill percentage}, then performs \textit{smoothing
iterations} that either fill an empty cell if the number of its filled neighbors is larger than \textit{fill threshold} or empty a filled cell if its filled neighbors is smaller than \textit{clear threshold}. The grids that are not navigable will be discarded. Due to the cellular automation, the resulting grid resembles real-world obstacles more than the initial randomly filled grid does. To generate BARN dataset, 12 different sets of hyper-parameters are used with \textit{initial fill percentage} chosen from $\{0.15, 0.2, 0.25, 0.3\}$ and \textit{smoothing
iterations} ranges from 2 to 4. The \textit{fill threshold} and \textit{clear threshold} are kept at 5 and 1 respectively. Each set of hyper-parameters generates 25 environments which constitute 300 environments in total. 
\begin{figure}
    \centering
    \includegraphics[width=0.9\textwidth]{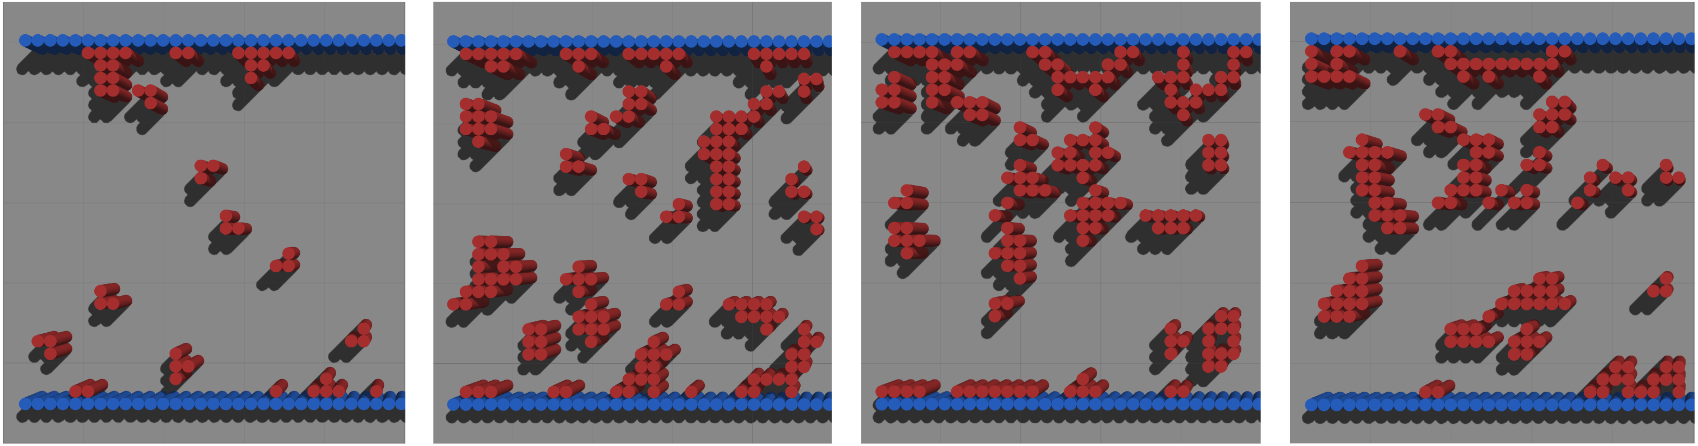}
    \caption{Examples of \texttt{static} environments.}
    \label{fig:static}
\end{figure}

\textbf{Dynamic box environments.}
These environments are $13.5m\times13.5m$ obstacle fields (larger than the static environments) that give the agent more time to respond to the moving obstacles (see Fig. \ref{fig:dynamic_box}). The obstacles are randomly generated without any manually designed challenging scenarios. Each obstacle is a $w\times l \times h$ box with its width $w$ and length $l$ randomly sampled from a range of $[0.1m, 0.5m]$ and a height $h=1m$. The obstacles start from a random position on the left edge of the obstacle field with a random orientation and a constant linear velocity. The magnitude of the velocity is randomly sampled from a range of $[1m/s, 1.5m/s]$, and the direction of the velocity is randomly sampled from all the possible directions pointing into the obstacle field. Each obstacle repeats its motion once it moves out of the obstacle field. Each dynamic box environment has 10 to 15 such randomly generated obstacles.
%We randomly generate 100 instances of such dynamic box environments with 50 as the training set and the remaining 50 as the test set, which we denote as \texttt{dynamic-box-train} and \texttt{dynamic-box-test} respectively.
\begin{figure*}[htb!]
    \centering
    \includegraphics[width=0.9\textwidth]{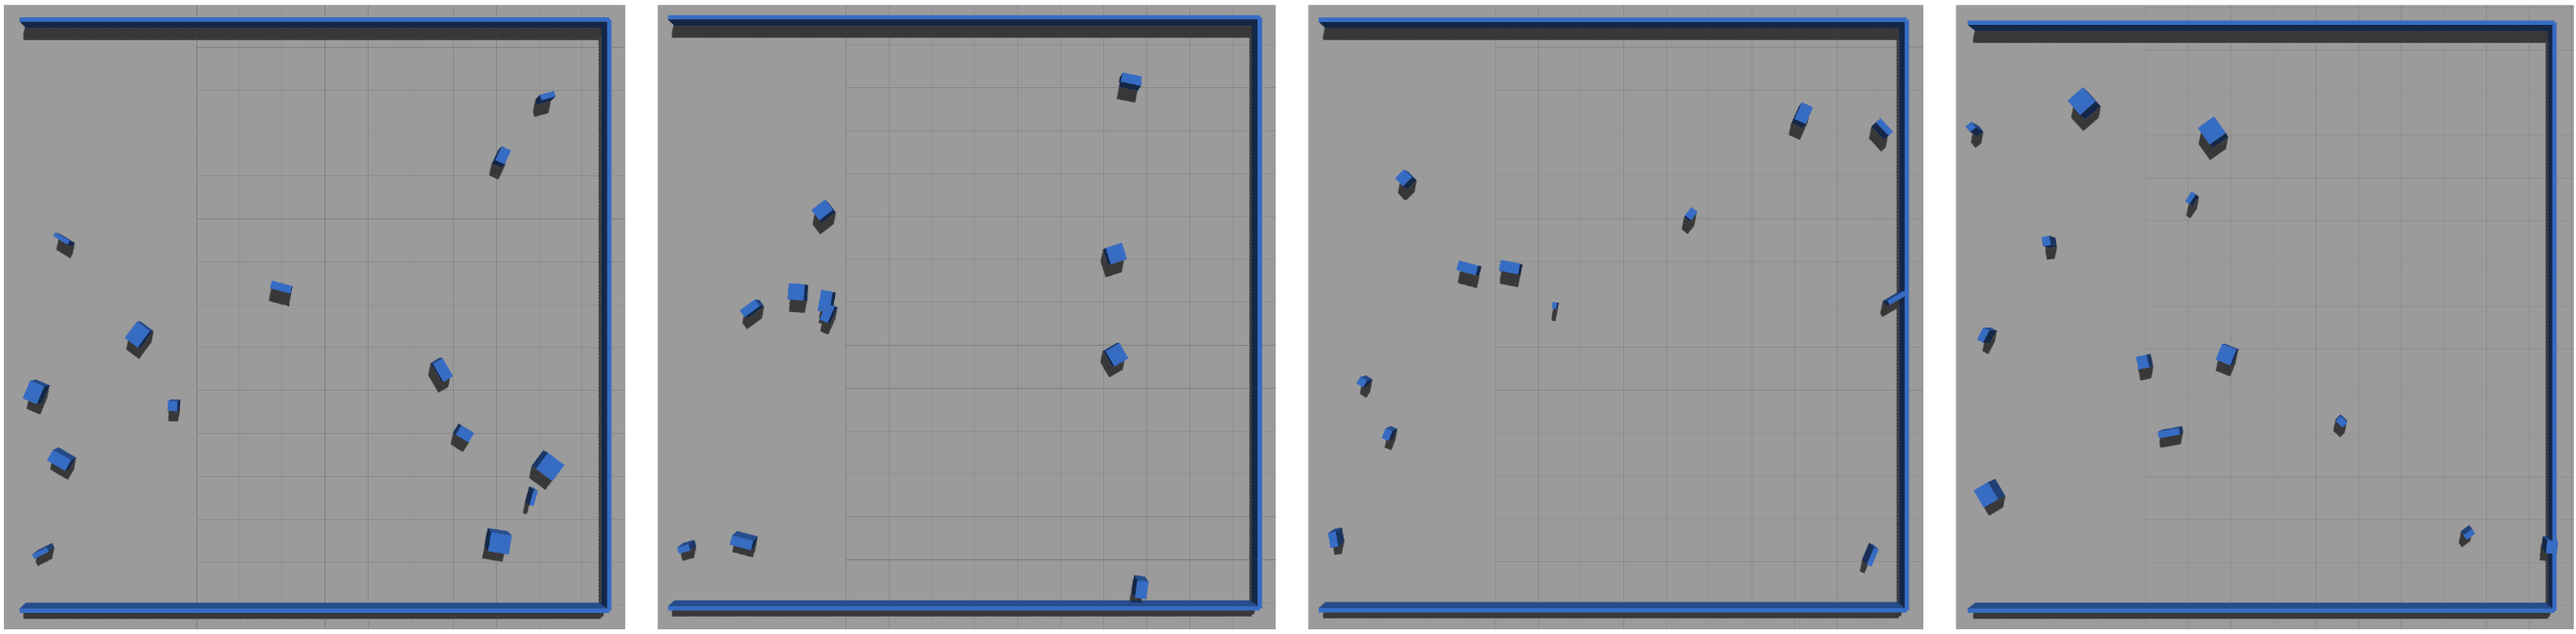}
    \caption{Examples of \texttt{dynamic-box} environments.}
    \label{fig:dynamic_box}
\end{figure*}

\begin{figure*}[htb!]
    \centering
    \includegraphics[width=0.9\textwidth]{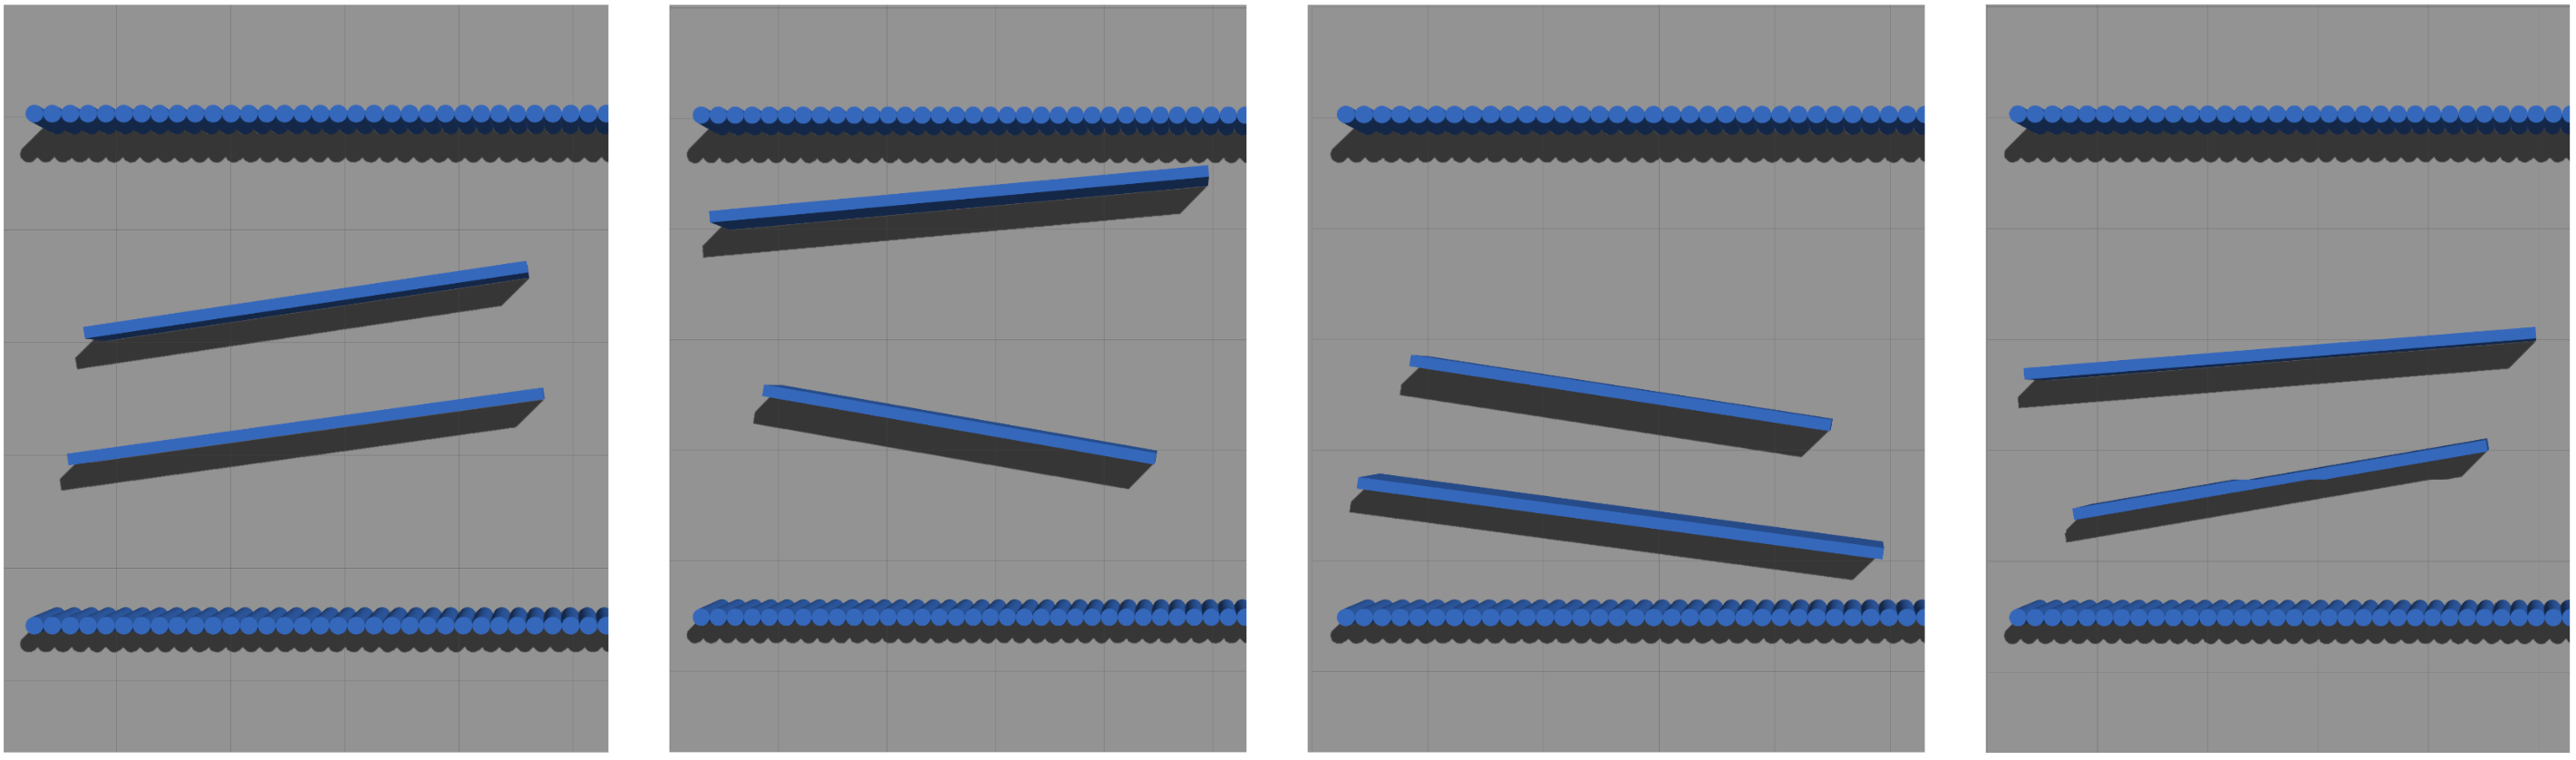}
    \caption{Examples of \texttt{dynamic-wall} environments.}
    \label{fig:dynamic_wall}
\end{figure*}

\textbf{Dynamic wall environments.}
These environments are $4.5m\times4.5m$, which have two long parallel walls moving in opposite directions with their velocities perpendicular to the start-goal direction (see Fig. \ref{fig:dynamic_wall}). The walls are long enough so that the robot can only pass when the two walls are moving apart. This manually designed navigation scenario requires the agent to maintain a memory of past observations and actions, and to estimate the motion of obstacles. To challenge the agent, we add small variances so that each wall's length, tilting angle, and magnitude of the velocity are randomly sampled from the ranges of $[3.5m, 4.5m]$, $[-10^{\circ}, 10^{\circ}]$ and $[1m/s, 1.4m/s]$ respectively.
