# Supplementary material for: Benchmarking Reinforcement Learning Techniques for Autonomous Navigation
Source: arXiv:2210.04839 source file (2023-06-27)
Supplement: Supplementary file 2 [file appendix_simulation_specification.tex]

\section{Jackal Robot and Navigation system}
\label{appendix:specifications}
As shown in Fig. \ref{fig:system} on the left, the navigation is performed by a ClearPath Jackal differential-drive ground robot in navigation environments simulated by the Gazebo simulator. The  robot is equipped with a 720-dimensional planar laser scan with a 270$^\circ$ field of view, which is used as our sensory input $\chi_t$. We preprocess the LiDAR scans by capping the maximum range to 5m which covers the entire obstacle field. The goal location $(\bar{x_t}, \bar{y_t})$ is queried directly from the Gazebo simulator. The robot receives velocity commands at a frequency of 5 Hz. A time limit of $80s$ is used which corresponds to a maximum of 400 time steps in an episode. In the real world, the robot is deployed in the same way as simulation except for that the goal location is queried from the on-board ROS \texttt{move\_base} stack \cite{ros_move_base} that localizes the robot simultaneously. Fig. \ref{fig:system} on the right shows a diagram of the RL-based navigation system.
\begin{figure*}
    \centering
    \includegraphics[width=0.9\textwidth]{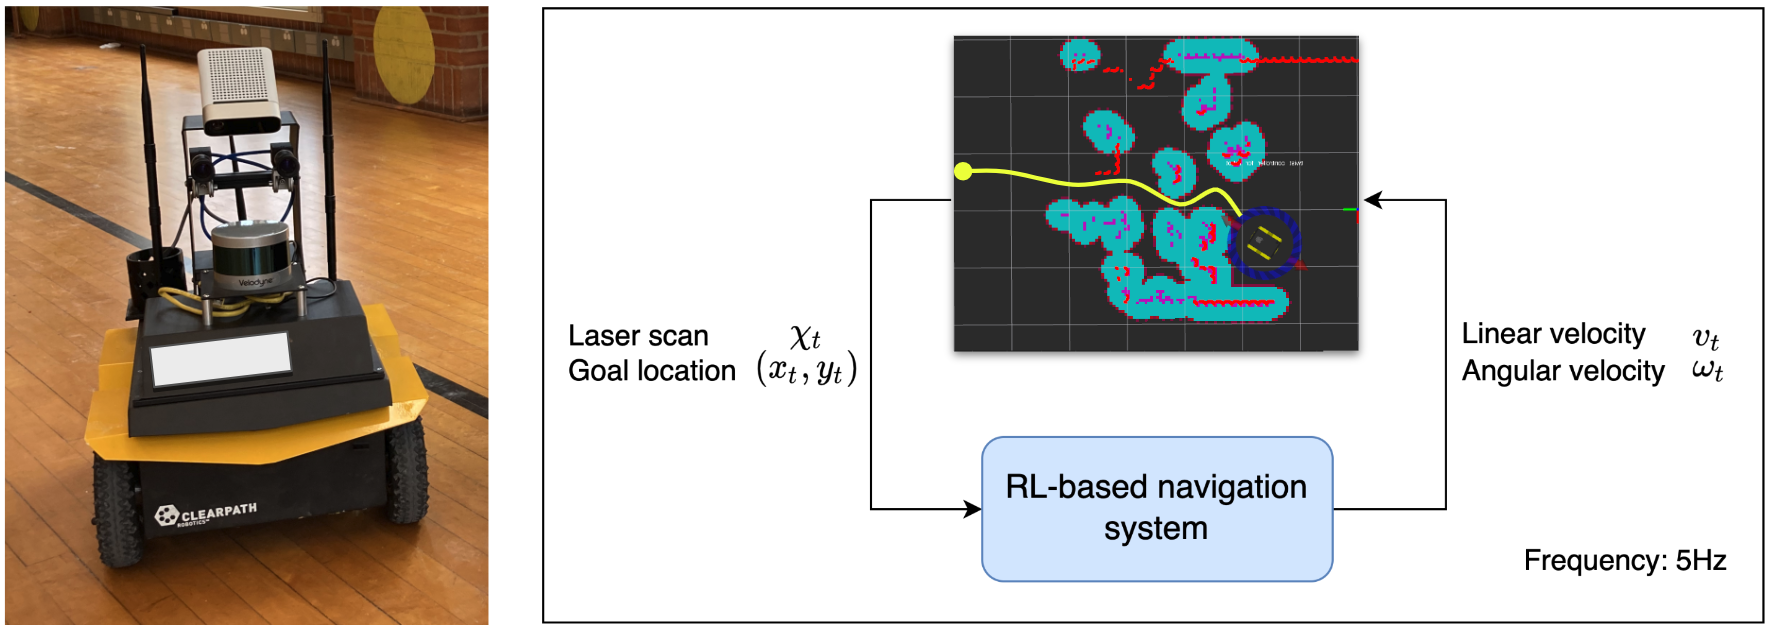}
    \caption{The picture of a Jackal Robot (left) and the diagram of the RL-based navigation system.}
    \label{fig:system}
\end{figure*}
