# Supplementary material for: Benchmarking Reinforcement Learning Techniques for Autonomous Navigation
Source: arXiv:2210.04839 source file (2023-06-27)
Supplement: Supplementary file 3 [file appendix_techniques.tex]

\section{Studied Techniques}
\label{appendix:techniques}
In Sec. \ref{subsec::mdp}, a brief review of Reinforcement Learning (RL) and Markov decision processes (MDPs) is provided. Then, Sec. \ref{sec:nn} to \ref{sec:dr} describes in detail the studied techniques and how they can potentially achieve the desiderata.

\subsection{RL and MDPs}
\label{subsec::mdp}
In RL, an agent optimizes its discounted cumulative return through interactions with an environment, which is formulated as an MDP. Specifically, an MDP is a 5-tuple $(S, A, T, \gamma, R)$, where $S, A$ are the state and action spaces, $T: S \times A \rightarrow S$ is the transition kernel that maps the agent's current state and its action to the next state, $\gamma$ is a discount factor and $R: S \times A \rightarrow \mathbb{R}$ is the reward function. The overall objective is for the agent to find a policy function $\pi: S \rightarrow A$ such that its discounted cumulative return is maximized: $\pi^* = \arg \max_\pi \mathbb{E}_{s_t, a_t \sim \pi} \big[\sum_{t=0}^\infty \gamma^t R(s_t, a_t)\big]$~\cite{sutton2018reinforcement}. %\xuesu{Do we need a citation for this?}

MDPs assume the agent has access to the world state $s$ which encapsulates sufficient information for making optimal decisions. However, in real applications, the agent often only perceives part of the state $s$ at any moment. Such partial observability leads to uncertainty in the world state and the problem becomes a Partially Observable Markov decision process (POMDP). A POMDP is a 7-tuple $(S, A, O, T, \gamma, R, Z)$. In addition to the elements of an MDP, $O$ denotes the observation space and $Z: S \rightarrow O$ is an observation model that maps the world state to an observation. For instance, at each time step $t$, the agent receives an observation $o_t \sim Z(\cdot \mid s_t)$. In general, solving a POMDP optimally requires taking the entire history into consideration, which means the objective is then to find a policy that maps its past trajectory $\tau_t = (o_0, a_0, \dots, o_t, a_t)$ to an action $a_t$ such that $\max_\pi \mathbb{E}_{\tau_t \sim \pi} \big[\sum_{t=0}^\infty \gamma^t R(s_t, a_t)\big]$.

\subsection{Memory-based Neural Network Architectures (D1)} 
\label{sec:nn}
Due to the uncertainty from partial observations (e.g., caused by dynamic obstacles or imperfect sensory inputs), a mobile agent often needs to aggregate the information along its trajectory history (as in many classical systems, a costmap is being continuously built based on previous perceptions). When using a parameterized model as the policy, recurrent neural networks (RNNs) such as those incorporating Long-Short Term Memory (LSTM)~\cite{hochreiter1997long} or Gated Recurrent Units (GRUs)~\cite{chung2014empirical} are widely adopted for solving POMDPs~\cite{Hausknecht2015DeepRQ, Wierstra2007SolvingDM}. More recently, transformers~\cite{vaswani2017attention}, a type of deep neural architecture that use multiple layers of attention mechanism to process sequence data, have been proposed. Transformers have demonstrated superior performance over RNN-based models in vision and natural language applications~\cite{vaswani2017attention}. In this work, we consider both GRU and transformers as the backbone model for the navigation policy. The reason for choosing GRU over LSTM is due to the fact that GRU has a simpler architecture than, but performs comparably with, LSTM in practice~\cite{chung2014empirical}.

\subsection{Safe RL (D2)}
\label{sec:saferl}
Successful navigation involves both navigating efficiently towards a user specified goal and avoiding collisions. While most prior RL-based navigation approaches design a \emph{single} reward function that summarizes both objectives, it is not clear whether explicitly treating the two objectives separately will have any benefits.
Specifically, assume the reward function $R$ only rewards the agent for making progress to the goal. Additionally, a cost function $C: S \times A\rightarrow \mathbb{R}^+$ maps a state $s$ and the agent's action $a$ to a penalty $c$. Then the navigation problem can be transformed into a constrained optimization problem with 2 objectives~\cite{altman1999constrained}:
\begin{equation}
    \max_\pi \mathbb{E}_{s_t, a_t \sim \pi} \bigg[\sum_{t=0}^\infty \gamma^tR(s_t, a_t)\bigg]~~~\text{s.t.}~~~ \mathbb{E}_{s_t, a_t \sim \pi} \bigg[\sum_{t=0}^\infty \gamma^t C(s_t, a_t)\bigg] \leq \epsilon.
    \label{eq:safe-rl}
\end{equation}
Here $\epsilon \geq 0$ is a threshold that controls how tolerant we are of the risk of collision. By formulating the navigation problem in this way, existing constrained optimization techniques can be applied for solving \eqref{eq:safe-rl}. One of the most common approaches in constrained optimization is using a Lagrangian multiplier, which transforms the constraint into a penalty term multiplied by a Lagrangian multiplier $\lambda \geq 0$. Specifically, the objective becomes
\begin{equation}
    \max_\pi \mathbb{E}_{s_t, a_t \sim \pi} \bigg[\sum_{t=0}^\infty \gamma^tR(s_t, a_t)\bigg] + \lambda \bigg(\mathbb{E}_{s_t, a_t \sim \pi} \bigg[\sum_{t=0}^\infty \gamma^t C(s_t, a_t)\bigg] - \epsilon\bigg).
    \label{eq:safe-rl-lagr}
\end{equation}
To solve \eqref{eq:safe-rl-lagr}, one can either manually specify a $\lambda$ based on prior knowledge or optimize $\lambda$ simultaneously~\cite{boyd2004convex}. In this work, we perform a grid search over $\lambda$ but fix it during learning.

% \bo{consider whether to include the 2nd approach}
% Another approach to solve \eqref{eq:safe-rl} is to directly optimize the return while respecting the cost constraint at each optimization step. Specifically, denote $J_R = \mathbb{E}_{s_t, a_t \sim \pi} \bigg[\sum_{t=0}^\infty \gamma^tR(s_t, a_t)\bigg]$ and $J_C = \mathbb{E}_{s_t, a_t \sim \pi} \bigg[\sum_{t=0}^\infty \gamma^t C(s_t, a_t)\bigg]$, then \bo{add citations and finish}

\subsection{Model-based RL (D2, D3)}
\label{sec:model_based}
Given an accurate model, model-based RL often benefits from better sample efficiency compared to model-free methods~\cite{atkeson1997comparison}. In addition to improved sample efficiency, prior work on model-based RL also reported that planning with a learned model can improve the agent's safety~\cite{thomas2022safe}.
Therefore, we investigate whether these claims also hold for autonomous navigation if the agent learns a transition model $\hat{T}$ from its interaction with the world. Although the reward model $R$ can also be learned, as the structure of the reward function is usually designed manually, we let the agent take advantage of the known reward function. In this work, we consider two ways of using a learned model: a Dyna-style method~\cite{sutton1990integrated} and model-predictive control (MPC)~\cite{rossiter2017model}. Specifically, assume the agent's rollout trajectories are saved into a replay buffer $B$ in the form of transition tuples: $B = \{(s_t, a_t, s_{t+1}, r_t)\}_t$.\footnote{Replay buffer is a commonly used technique to learn the value function (critic) in reinforcement learning.} Then model-based methods assume the agent also learns a model $\hat{T}: S \times A \rightarrow S$ that approximates $T$. A common learning objective of $\hat{T}$ is to minimize the mean-square-error between $\hat{T}$'s and $T$'s predictions on transitions:
\begin{equation}
    \hat{T} = \argmin_{T'}~~\mathbb{E}_{(s,a,s',r) \sim B}\big|\big| T'(s, a) - s'\big|\big|_2^2. 
\end{equation}
Once $\hat{T}$ is learned, given a transition pair $(s,a) \sim B$, the Dyna-style method samples additional $s' \sim \hat{T}(s, a)$ to enrich the replay buffer that can potentially benefit the learning of the value function. MPC, on the other hand, first uses $\hat{T}$ to form samples of future trajectories, then it outputs the first action corresponding to the trajectory that has the highest return. MPC usually enables a more efficient exploration by selecting promising actions, and also potentially improves the asymptotic performance with the help of model predictions.

\subsection{Domain randomization (D4)} 
\label{sec:dr}
A direct deployment of a policy trained in limited training environments to unseen target environments is usually formalized as a zero-shot transfer problem, where no extra training of the policy is allowed in the target environments. One promising approach for zero-shot transfer has been Domain Randomization (DR) \cite{tobin2017domain}. In DR, the environment parameters (i.e. obstacle configurations) in predefined ranges are randomly selected in each training environment. By randomizing everything that might vary in the target environments, the generalization can be improved by covering target environments as variations of random training environments. This simple yet strategy has been reported to be efficient in practice when solving many sim-to-real transfer problems \cite{tobin2017domain, Sadeghi2017CAD2RLRS, Peng2018SimtoRealTO}.
